# Supplementary material for: Information-theoretic limits of a multiview low-rank symmetric spiked matrix model
Source: arXiv:2005.08017 source file (2020-05-16)
Supplement: Supplementary file 1 [file appendix.tex]

\subsection{Nishimori identity}\label{appendix:nishimori}

\begin{lemma}\label{prop:nishimori}
	Let $(X,Y)$ be a couple of random variables on a polish space $E$. For a given $k \in \mathbb{N}^*$, let $(X^{(i)})_{i=1}^k$ be i.i.d random variables from the distribution (conditional over $Y$) $P(X = \cdot|Y)$. Denote $\langle - \rangle$ the expectation with respect to this probability distribution, and $\EE$ the expectation with respect to the probability measure of $(X,Y)$. Then, for all $f : E^{k+1} \to \mathbb{R}$ continuous and bounded
	\begin{align*}
	\EE \langle f(Y,X^{(1)},\ldots,X^{(k)})  \rangle = \EE \langle f(Y,X^{(1)},\ldots,X^{(k-1)},X)  \rangle\,.
	\end{align*}
\end{lemma}

\begin{IEEEproof}
This is a trivial consequence of Bayes formula: 
\begin{align*}
\EE_{X,Y} \langle f(Y,X^{(1)},\cdots,X^{(k-1)},X) \rangle &= \EE_{Y} \EE_{X|Y} \langle f(Y,X^{(1)},\cdots,X^{(k-1)},X) \rangle\\
&= \EE \langle f(Y,X^{(1)},\cdots,X^{(k)})\rangle\,.
\end{align*}
\end{IEEEproof}

\subsection{Proof of Lemma~\ref{lemma:derivative}}\label{appendix:proof_derivative}

The proof is done in two steps. First, we show the following formula:
\begin{align}\label{eq:derivative_first_step}
&i_n'(t) = \frac{r}{2} (\rho - \EE \langle Q \rangle_t) + \frac{1}{2n^2}  \sum_{\mu=1}^m \sum_{\nu=1}^m  \EE  \Big\langle Z_\mu (\bm{\Phi'} \bm{\Phi'}^\intercal)_{\mu \nu} u_{t,\nu} \Big[E(t) - \Big(\frac{1}{n}\sum_{i=1}^n X_i^2 - Q \Big) \Big] \Big\rangle_t \,.
\end{align}
We will then conclude using the concentration of $\frac{1}{n} \sum_{i=1}^n X_i^2$ on $\rho$ by the central limit theorem as $n \to \infty$. 

Recall that we defined the Gibbs bracket 
\begin{align}
\langle A(\bx,\bv)\rangle_t = \frac{\int dP_0(\bx) {\cal D}\bv e^{-{\cal H}(t,\bx,\bv;\bY_t,\widetilde \bY_t,\bm{\Phi})} A(\bx,\bv)}{\int dP_0(\bx) {\cal D}\bv e^{-{\cal H}(t,\bx,\bv;\bY_t,\widetilde \bY_t,\bm{\Phi})}}\,.
\end{align}
From this and the definition of $i_n(t)$ (\ref{eq:def_mutual_info}), one gets
\begin{align}\label{eq:in_derivative}
i_n'(t) = \frac{1}{n}\EE\big[ {\cal H}'(t,\bX,\bV;\bY_t,\widetilde \bY_t,\bm{\Phi})\ln {\cal Z}\big]+
\frac{1}{n}\mathbb{E}\big\langle {\cal H}'(t,\bx,\bv;\bY_t,\widetilde \bY_t,\bm{\Phi})\big\rangle_t\,,
\end{align}
where the partition function $\cal Z$ and Hamiltonian derivatives read
\begin{align}
{\cal H}'(t,\bX,\bV;\bY_t,\widetilde \bY_t,\bm{\Phi})
&=\frac{1}{2}\sum_{\mu=1}^m Z_\mu\Big(\sqrt{\frac{1}{n(1-t)}}(\bm{\Phi}\bX)_\mu - \frac{ E(t)}{\sqrt{n\widetilde E(t)}} (\bm{\Phi'} \bV)_\mu\Big)-\frac12 \sum_{i=1}^n\widetilde Z_i \sqrt{\frac{r}{t}}X_i \,,\\
{\cal Z}={\cal Z}(t,\bY_t,\widetilde \bY_t,\bm{\Phi})&\equiv\int dP_0(\bx) {\cal D}\bv e^{-{\cal H}(t,\bx,\bv;\bY_t,\widetilde \bY_t,\bm{\Phi})}\,.
\end{align}

The Nishimori identity Lemma~\ref{prop:nishimori} directly implies  
\begin{align}
\mathbb{E}\big\langle {\cal H}'(t,\bx,\bv;\bY_t,\widetilde \bY_t,\bm{\Phi})\big\rangle_t = \mathbb{E} {\cal H}'(t,\bX,\bV;\bY_t,\widetilde \bY_t,\bm{\Phi}) = 0\,.
\end{align}

We now compute $\EE[ \widetilde Z_iX_i\ln {\cal Z}]$. Using a Gaussian integration by parts, which reads for any real function $f$ with continuous derivative $\EE[\widetilde Z_if(\widetilde Z_i)]=\EE[f'(\widetilde Z_i)]$ for $\widetilde Z_i \sim {\cal N}(0,1)$, we obtain the first term of \eqref{eq:in_derivative} as
	\begin{align}		
		&-\frac1{2n}\sqrt{\frac{r}{t}}\sum_{i=1}^n\EE \Big[X_i \widetilde Z_i \ln \int dP_0(\bx) {\cal D}\bv e^{-{\cal H}(t,\bx,\bv;\bY_t,\widetilde \bY_t,\bF)}  \Big]\nonumber\\
		=~&-\frac1{2n}\sqrt{\frac{r}{t}}\sum_{i=1}^n\EE \Big[X_i \widetilde Z_i \ln \int dP_0(\bx) {\cal D}\bv\, 
		e^{
			{\text{term}}_1(\bv,\bx)- \frac{1}{2} \sum_i\big(\sqrt{tr}(X_{i}-x_i) + \widetilde Z_i \big)^2
		}  
	\Big]\nonumber \\
		=~& \frac1{2n}\sqrt{\frac{r}{t}}\sum_{i=1}^n\EE \big[X_i \big\langle \sqrt{tr}(X_i - x_i) +\widetilde Z_i \big\rangle_t \big]
	\nn
	=~& \frac{r\rho}{2}-\frac{r}{2}
		\EE 
		\Big\langle
			\frac1n\sum_{i=1}^{n} X_i x_i
		\Big\rangle_t \nonumber\\
		=~ &\frac{r}{2}(\rho-
		\EE \langle Q \rangle_t)\,.
	\end{align}
% Thus, by taking the sum, one computes . This leads to
% 	\begin{align}\label{eq:derivative_term_1}
% 		-\frac12\sqrt{\frac{r}{t}}\EE\Big[ \frac1n \sum_{i=1}^{n} X_i \widetilde Z_i\ln {\cal Z}  \Big]
% 		= \frac{r\rho}{2}-\frac{r}{2}
% 		\EE 
% 		\Big\langle
% 			\frac1N\sum_{i=1}^{N} X_i x_i
% 		\Big\rangle_t = \frac{r\rho}{2}-\frac{r}{2}
% 		\EE \langle Q \rangle_t\,.
% \end{align}
%
In the same way, an integration by parts with respect to $V_i \sim \mathcal{N}(0,1)$ yields 
\begin{align}\label{eq:derivative_term_2}
	&-\frac1{2n}\frac{E(t)}{\sqrt{n\widetilde E(t)}}\sum_{\mu=1}^m\EE\Big[ Z_\mu (\bm{\Phi'} \bV)_\mu \ln {\cal Z}\Big]\nonumber\\ 
=~ &-\frac1{2n}\frac{E(t)}{\sqrt{n\widetilde E(t)}}\sum_{\mu=1}^m \sum_{i=1}^n\EE\Big[ Z_\mu \Phi'_{\mu i} V_i  \ln\int dP_0(\bx){\cal D}\bv e^{-\frac12 \sum_{\nu} \big(\sqrt{\frac{1-t}{n}} (\bm{\Phi}(\bX-\bx))_\nu + \sqrt{\frac{\widetilde E(t)}{n}} (\bm{\Phi}'(\bV-\bv))_\nu+Z_\nu \big)^2+{\text{term}}_2(\bx)}\Big] \nonumber \\
	=~ &\frac{1}{2n^2} E(t) \sum_{\mu=1}^m \sum_{\nu=1}^m \sum_{i=1}^n\EE\Big[  Z_\mu \Phi'_{\mu i} \Phi'_{\nu i}\Big\langle\sqrt{\frac{1-t}{n}} (\bm{\Phi}(\bX-\bx))_\nu + \sqrt{\frac{\widetilde E(t)}{n}} (\bm{\Phi'}(\bV-\bv))_\nu+Z_\nu  \Big\rangle_t\Big] \nonumber \\
	 =~ &\frac{1}{2n^2} E(t) \sum_{\mu=1}^m \sum_{\nu=1}^m\EE\Big[   Z_\mu (\bm{\Phi'} \bm{\Phi'}^\intercal)_{\mu \nu}\langle u_{t,\nu} \rangle_t\Big]\,.
\end{align}
Let us now look at the final term we need to compute. By our hypothesis \eqref{eq:decomposition}, this term reads, using again a Gaussian integration by part but this time with respect to $W_{ji}\sim{\cal N}(0,1/n)$, 
\begin{align*}
&\frac{1}{2n}\sqrt{\frac{1}{n(1-t)}} \sum_{\mu=1}^m\EE\Big[Z_\mu(\bm{\Phi'} \bW \bX)_\mu \ln{\cal Z}\Big] \nonumber\\
= ~ & \frac1{2n} \sqrt{\frac{1}{n(1-t)}}\sum_{\mu=1}^m\sum_{i,j=1}^n\EE\Big[Z_\mu \Phi'_{\mu j}W_{ji} X_i \ln\int dP_0(\bx){\cal D}\bv e^{-\frac12 \sum_{\nu} \big(\sqrt{\frac{1-t}{n}} (\bm{\Phi'\bW}(\bX-\bx))_\nu + \sqrt{\frac{\widetilde E(t)}{n}} (\bm{\Phi}'(\bV-\bv))_\nu+Z_\nu \big)^2+{\text{term}}_2(\bx)}\Big]\nonumber\\
= ~ & -\frac1{2n^3}\sum_{\mu,\nu=1}^m\sum_{i,j=1}^n\EE\Big[Z_\mu \Phi'_{\mu j}\Phi'_{\nu j} X_i \Big\langle(X_i-x_i)\Big(\sqrt{\frac{1-t}{n}} (\bm{\Phi}(\bX-\bx))_\nu + \sqrt{\frac{\widetilde E(t)}{n}} (\bm{\Phi'}(\bV-\bv))_\nu+Z_\nu\Big)  \Big\rangle_t\Big]\nonumber\\
= ~ & -\frac1{2n^2}\sum_{\mu,\nu=1}^m\EE\Big[Z_\mu  (\bm{\Phi'} \bm{\Phi'}^\intercal)_{\mu \nu} \Big\langle u_{t,\nu}\Big(\frac1n\sum_{i=1}^n X_i^2 - \frac1n\sum_{i=1}^n X_ix_i \Big) \Big\rangle_t\Big]\,.
\end{align*}
Combining all three terms leads to \eqref{eq:derivative_first_step}.

We now go to the last step. By adding and substracting a term to \eqref{eq:derivative_first_step} we reach
\begin{align}\label{eq:derivative_second_step}
i_n'(t) = &\frac{r}{2} (\rho - \EE \langle Q \rangle_t) + \frac{1}{2n^2}  \sum_{\mu=1}^m \sum_{\nu=1}^m  \EE  \big\langle Z_\mu (\bm{\Phi'} \bm{\Phi'}^\intercal)_{\mu \nu} u_{t,\nu} \big[E(t) - (\rho - Q ) \big] \big\rangle_t \nn
&+\frac{1}{2n^2}  \sum_{\mu=1}^m \sum_{\nu=1}^m  \EE  \Big\langle Z_\mu (\bm{\Phi'} \bm{\Phi'}^\intercal)_{\mu \nu} u_{t,\nu} \Big(\rho - \frac{1}{n}\sum_{i=1}^n X_i^2 \Big) \Big\rangle_t \,.
\end{align}
Using the Cauchy-Schwarz inequality we obtain that the last term can be bounded as
\begin{align}
\frac1{n^2}\Big| \EE  \Big\langle \bZ^{\intercal} (\bm{\Phi'} \bm{\Phi'}^\intercal) \bu_{t} \Big(\rho - \frac{1}{n}\sum_{i=1}^n X_i^2 \Big) \Big\rangle_t\Big| \le \Big\{ \frac1{n^4}\EE  \Big\langle \Big(\bZ^{\intercal} (\bm{\Phi'} \bm{\Phi'}^\intercal) \bu_{t}\Big)^2\Big\rangle_t \EE\Big[\Big(\rho - \frac{1}{n}\sum_{i=1}^n X_i^2 \Big)^2\Big] \Big\}^{1/2}\,.\label{33}
\end{align}
As the $X_i$ are independent the central limit theorem implies that $\EE[(\rho - \frac{1}{n}\sum_{i=1}^n X_i^2 )^2]={\cal O}(1/n)$. Thus it remains to show that the multiplicative term in front is bounded:
\begin{align}
&\frac1{n^4}\EE  \big\langle\big( \bZ^{\intercal} (\bm{\Phi'} \bm{\Phi'}^\intercal) \bu_{t}\big)^2\big\rangle_t \le \frac{1}{n^4}\EE\big\langle \|\bZ\|^2 \|\bu_t\|^2 \|\bm{\Phi'} \bm{\Phi'}^\intercal\|_{\rm F}^2\rangle_t \nn
\le~& \frac{1}{n^4}\sqrt{\EE\big\langle \|\bZ\|^4 \|\bu_t\|^4\big\rangle_t \EE\big[ \|\bm{\Phi'} \bm{\Phi'}^\intercal\|_{\rm F}^4\big]}
\le\frac{1}{n^4}\sqrt{\sqrt{\EE\big[ \|\bZ\|^8\big]\EE\big\langle \|\bu_t\|^8\big\rangle_t}  \EE\big[ \|\bm{\Phi'} \bm{\Phi'}^\intercal\|_{\rm F}^4\big]}={\cal O}(1)\,. \label{34}
\end{align}
The last equality follows from the following observations. By construction of $\bm{\Phi'}$, $\EE[ \|\bm{\Phi'} \bm{\Phi'}^\intercal\|_{\rm F}^4]^{1/2} = {\cal O}(n^2)$. Moreover, as $\bZ$ is a $m$-dimensional Gaussian vector with i.i.d. components $\EE[ \|\bZ\|^8]^{1/4}={\cal O}(n)$. Finally, the Nishimori identity leads to $\EE[\langle\|\bu_t\|^8\rangle_t]^{1/4}={\cal O}(n)$. This claim is proven using a consequence the triangle inequality:
\begin{align*}
\forall \bx,\by \in \mathbb{R}^n \qquad \|x+y\|^8 \leq 2^7 (\|x^8\| + \|y^8\|)\,,
\end{align*}
which is combined with the Nishimori identity: 
\begin{align}
\EE[\langle\|\bu_t\|^8\rangle_t] =&~	\EE\Big\langle\Big\|\sqrt{\frac{1-t}{n}} \bm{\Phi}(\bX-\bx) + \sqrt{\frac{\widetilde E(t)}{n}} \bm{\Phi'}(\bV-\bv)+\bZ\Big\|^8\Big\rangle_t \nn
\le&~ 2^7 \EE[ \|\bZ\|^8] + 2^{22}(1-t)^4\EE[ \|\frac{1}{\sqrt{n}}\bm{\Phi}\bX \|^8] + 2^{22}\widetilde E(t)^4\EE[\| \frac{1}{\sqrt{n}}\bm{\Phi'}\bV\|^8]\,.\label{35}
\end{align}

One can now use that both $\frac{1}{n} \bm{\Phi}^\intercal\bm{\Phi}$ and $\frac{1}{n} \bm{\Phi'}^\intercal\bm{\Phi'}$ have almost surely bounded Euclidian (or Frobenius) norm when $n \to \infty$. This implies that there exists $C > 0$ such that
\begin{align*}
\EE[ \|\frac{1}{\sqrt{n}}\bm{\Phi}\bX \|^8] \leq C \EE[ \|\bX \|^8] \,.
\end{align*}
Moreover $\EE[ \|\bX \|^8] = {\cal O}(n^4)$ because we assumed the prior distribution $P_0$ to be compactly supported. The same argument can be conducted for bounding $\EE[ \|\frac{1}{\sqrt{n}}\bm{\Phi'}\bV \|^8]$ since $\EE[ \|\bV \|^8] = {\cal O}(n^4)$ as $\bV$
 is a standard Gaussian vector.
